# Supplementary material for: Vanadium in Silicon Carbide: Telecom-ready spin centres with long relaxation lifetimes and hyperfine-resolved optical transitions
Source: arXiv:2206.06240 source file (2022-06-13)

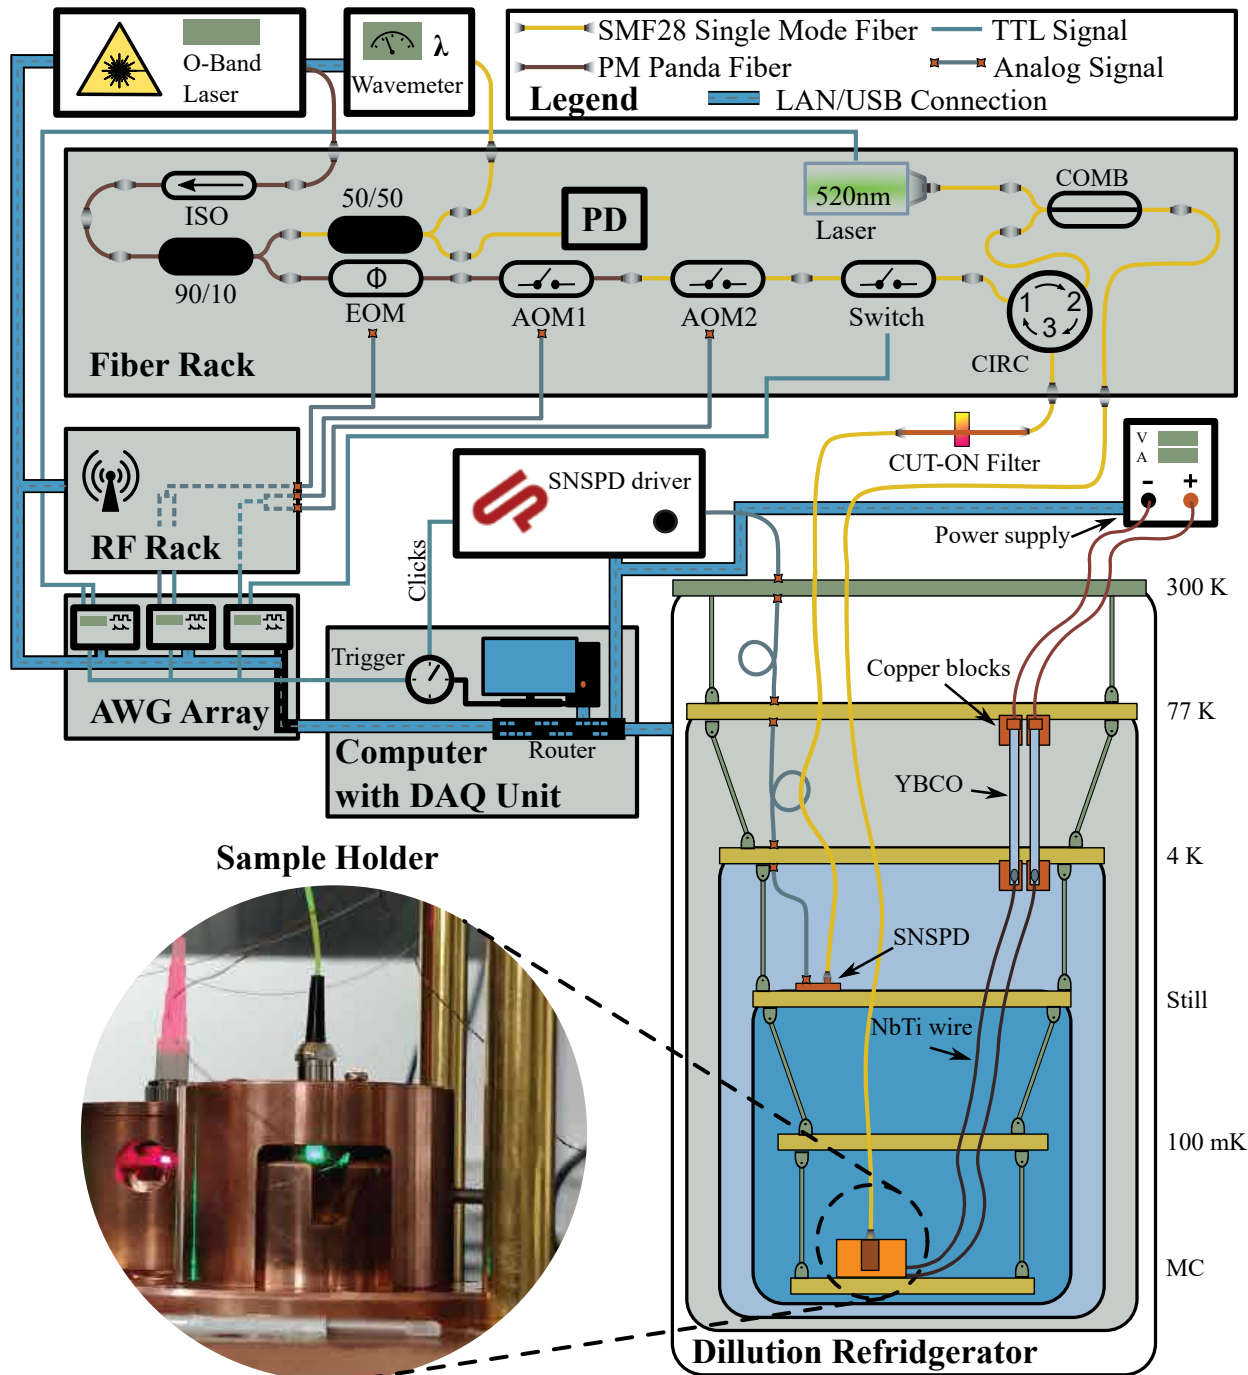

a)

### F-2F Spectroscopy

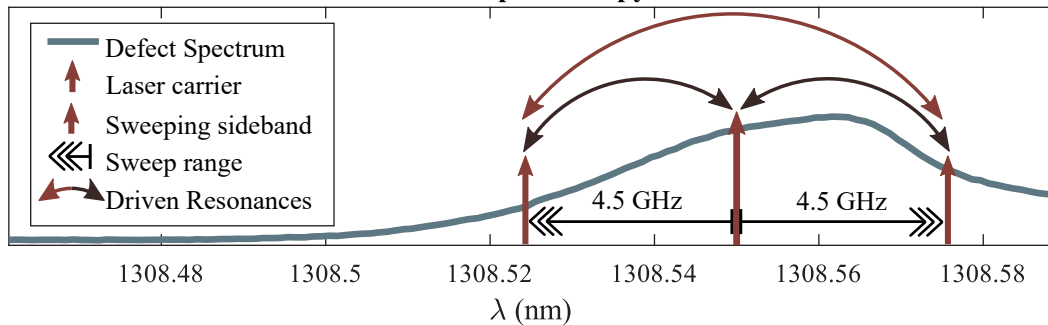

b)

### F-F Spectroscopy

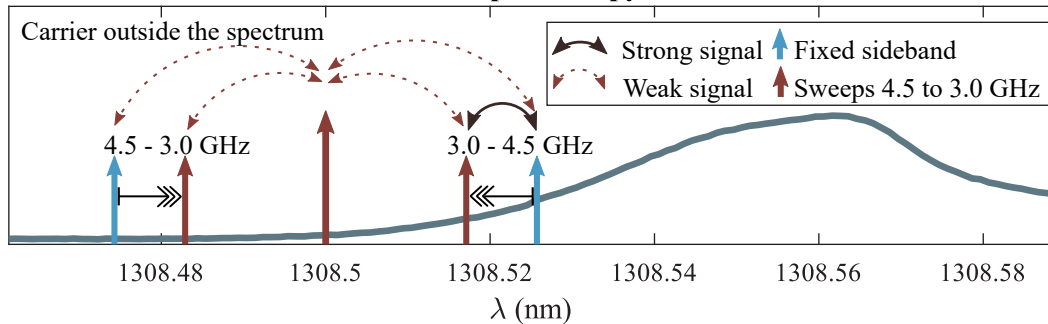

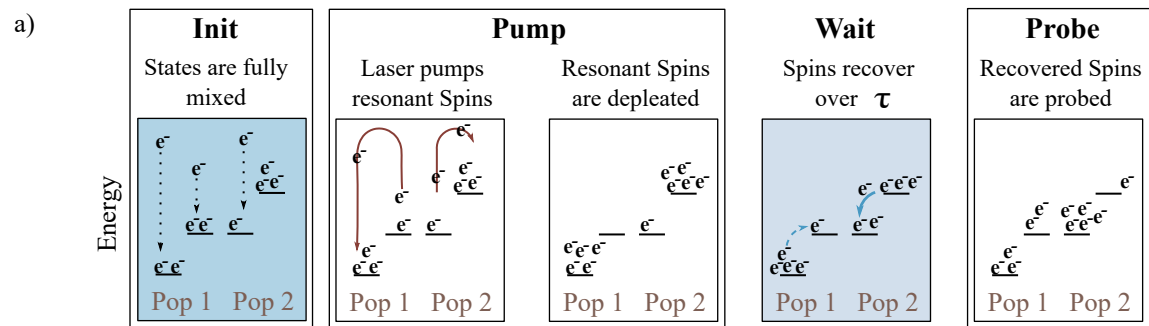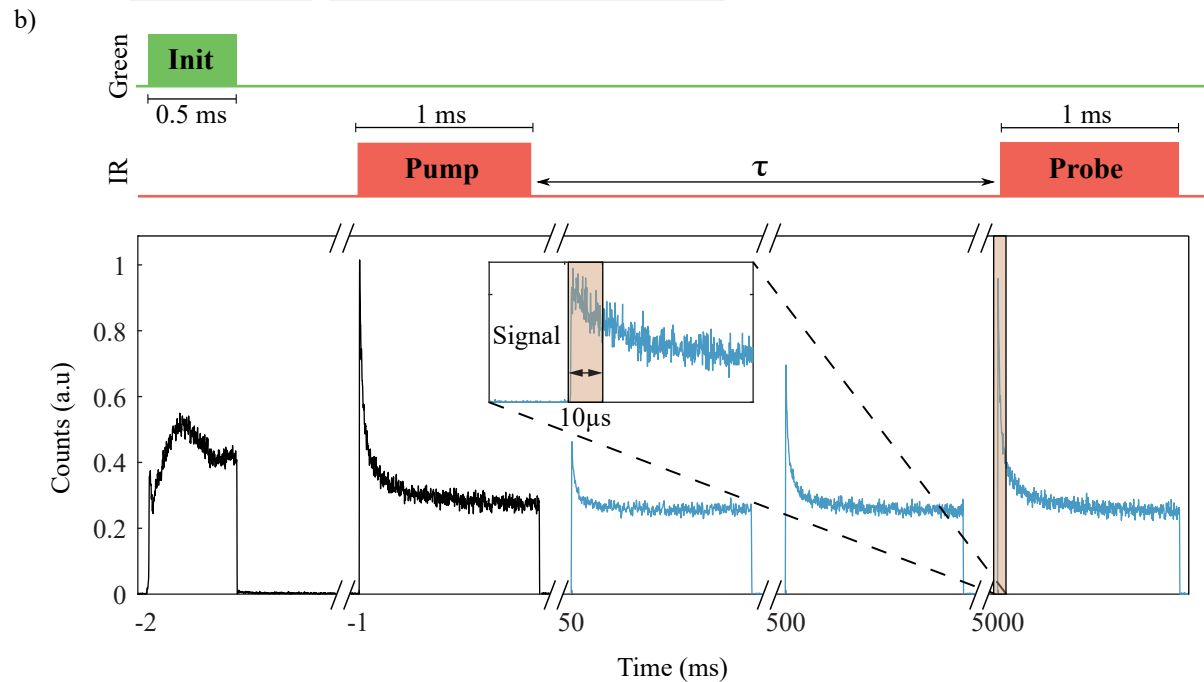

a)

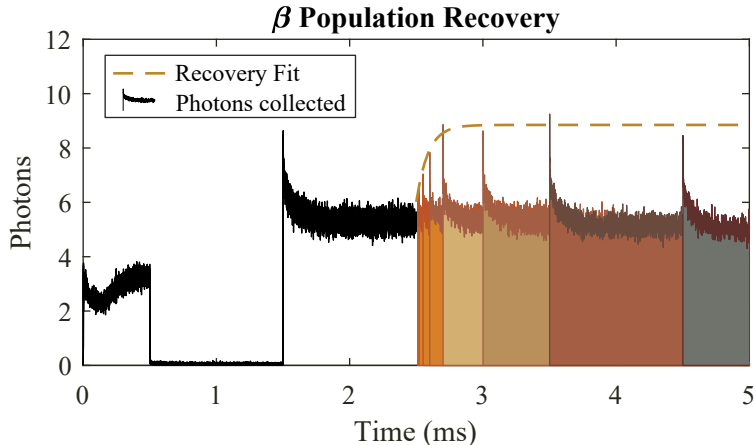

b)

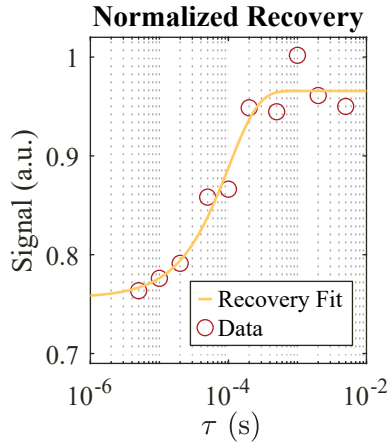

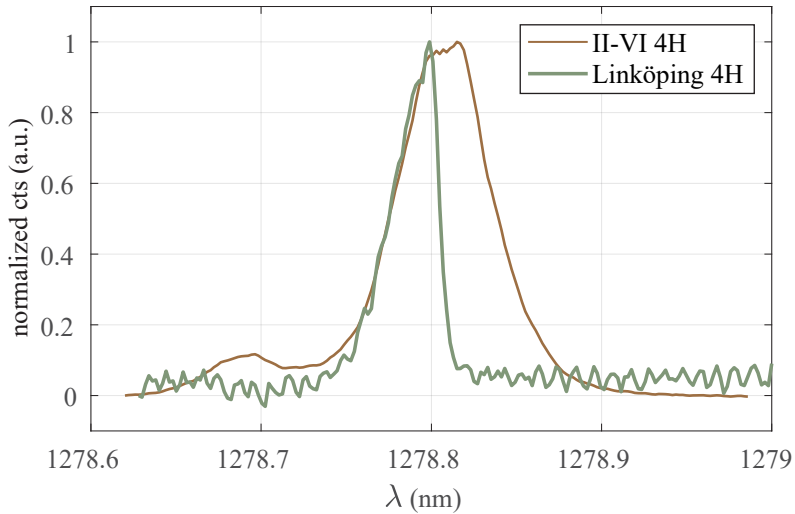

a)

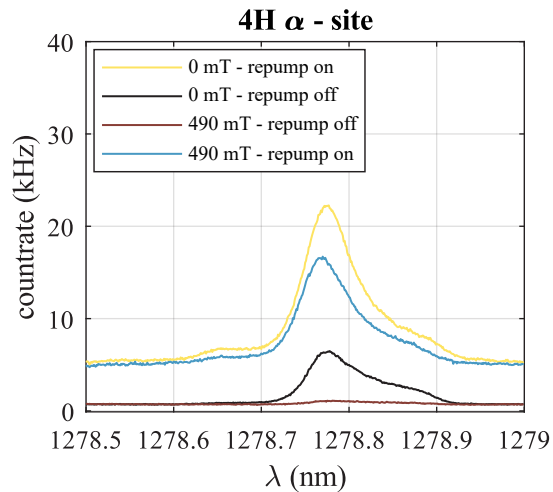

b)

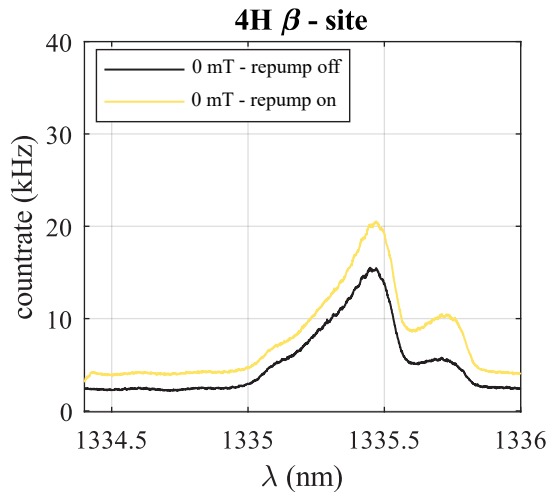

c)

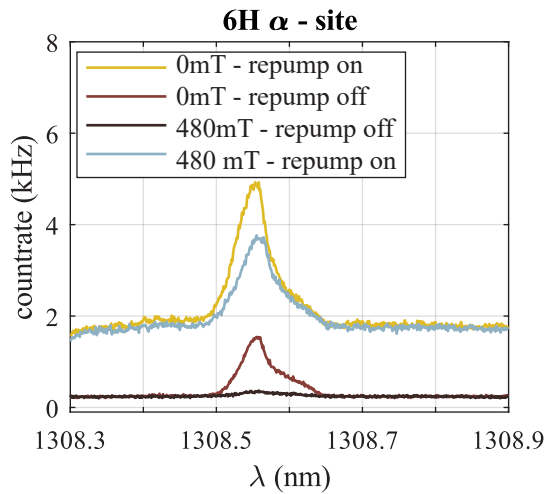

a)

**6H  $\alpha$  - site**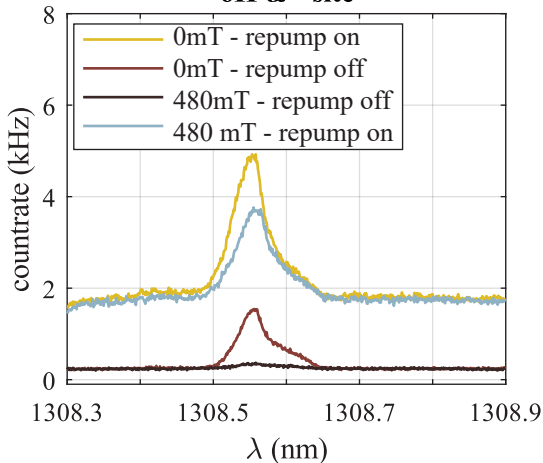

a)

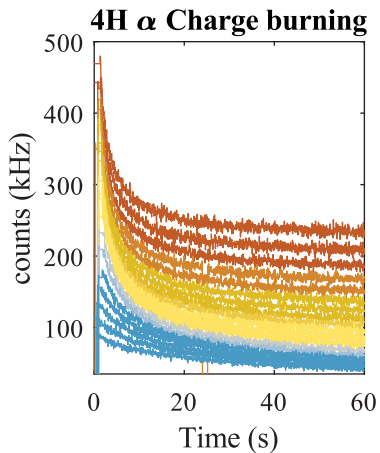

b)

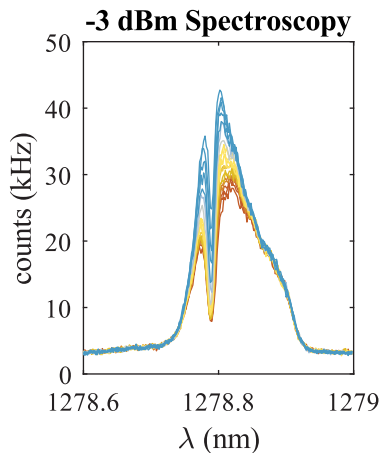

c)

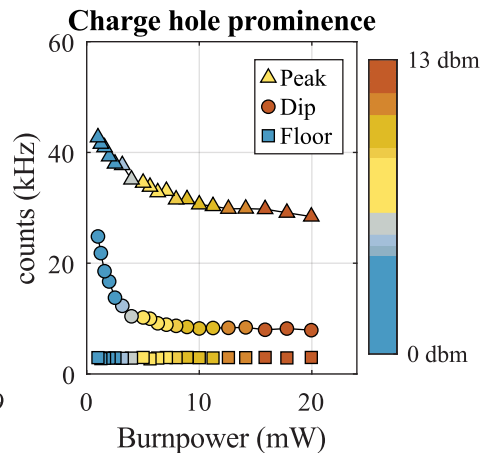

d)

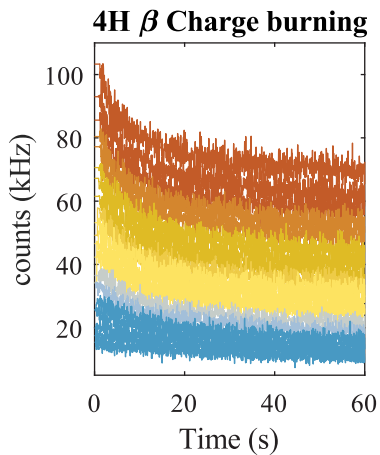

e)

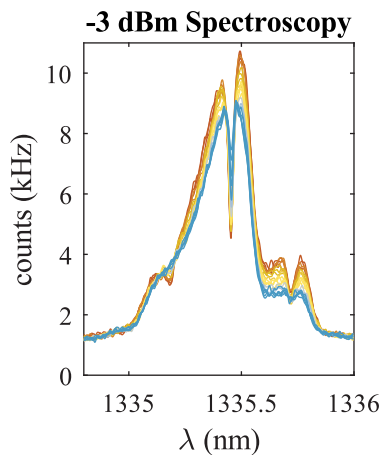

f)

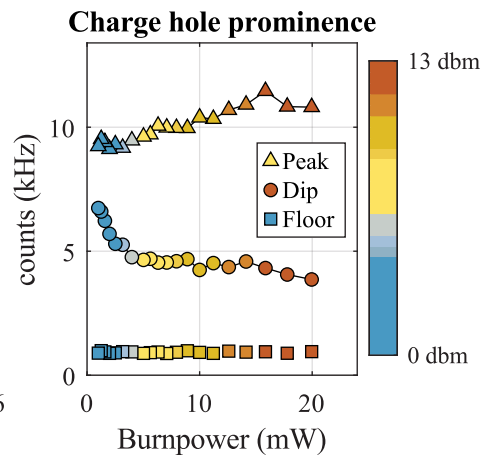



a)

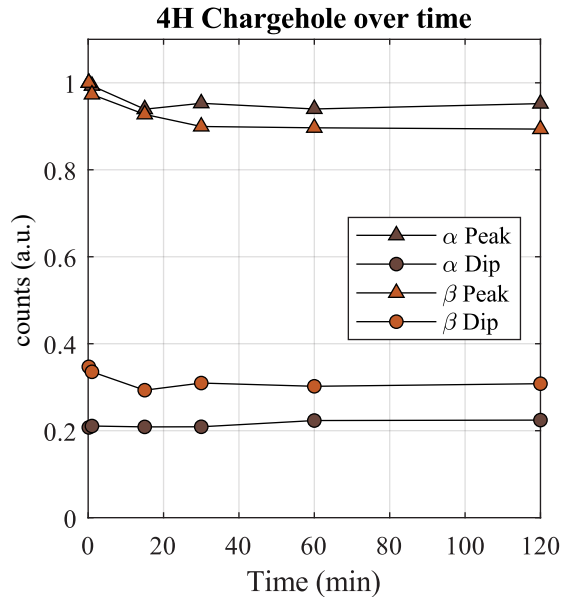

b)

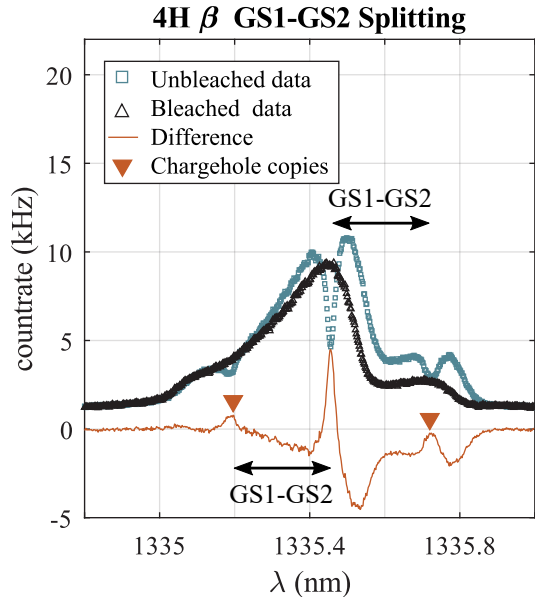

4H- $\beta$  low field

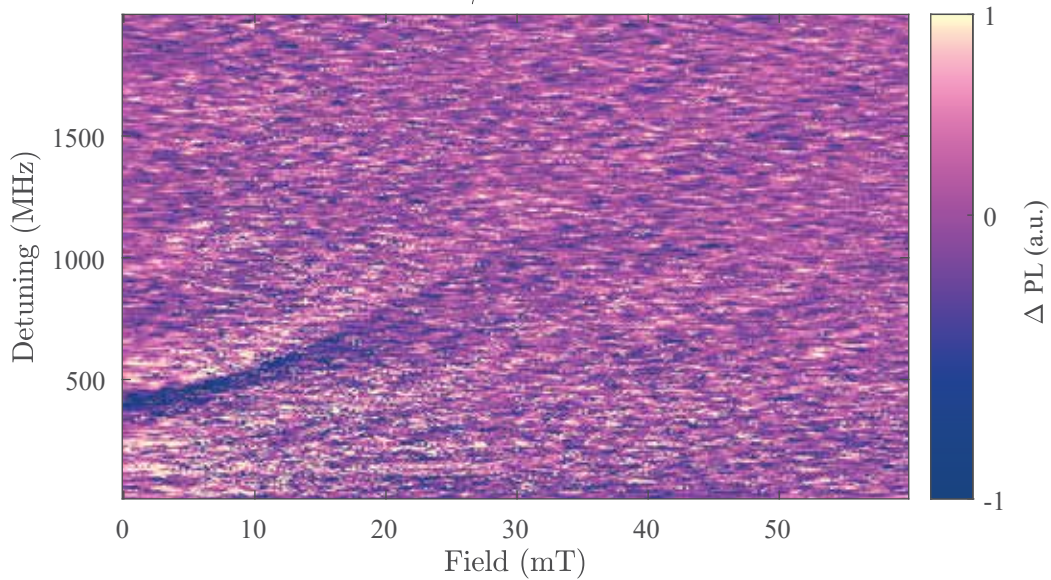

a)

6H- $\alpha$  low field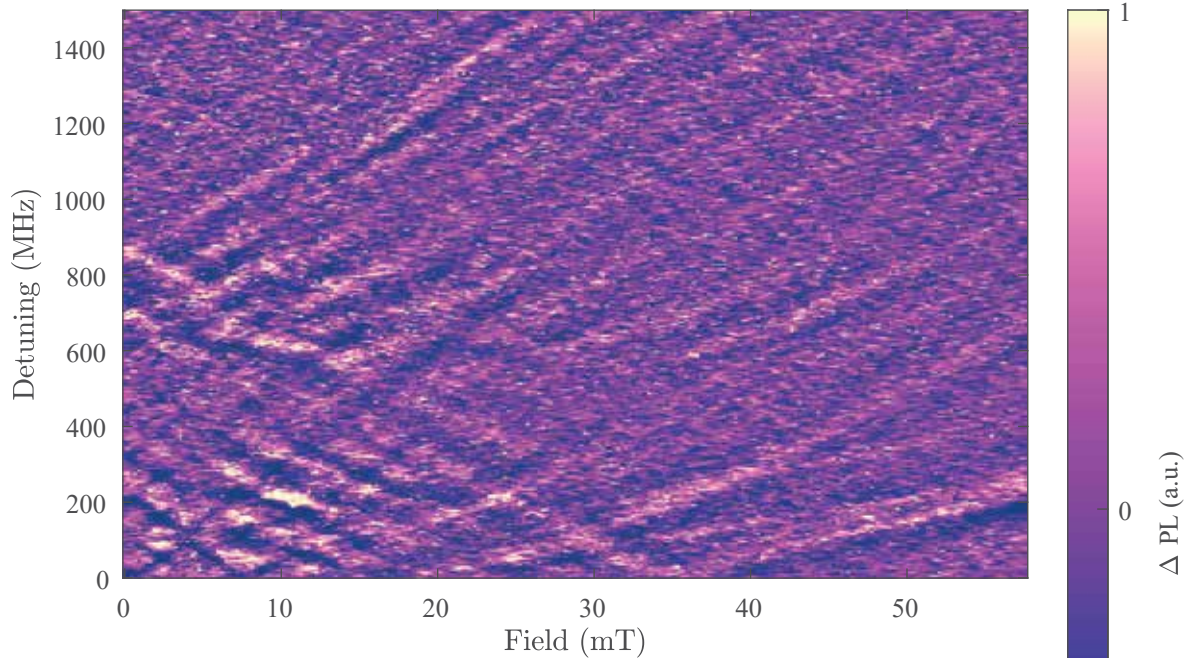

b)

6H- $\alpha$  high field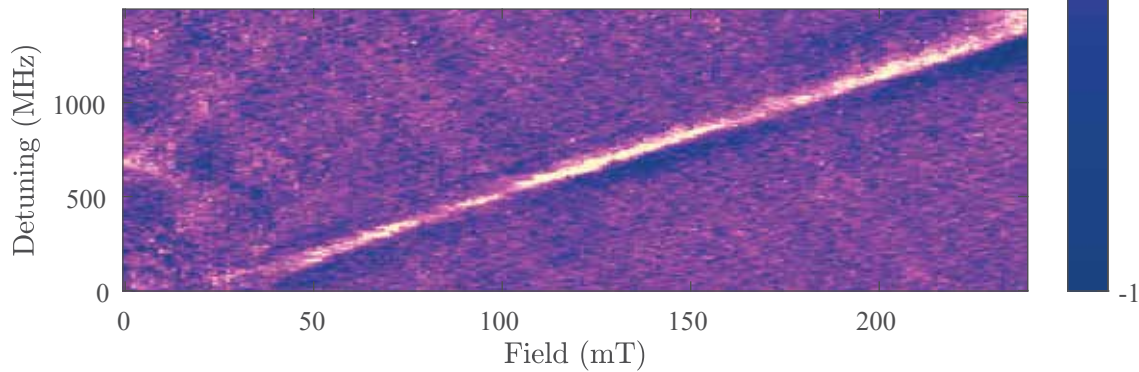

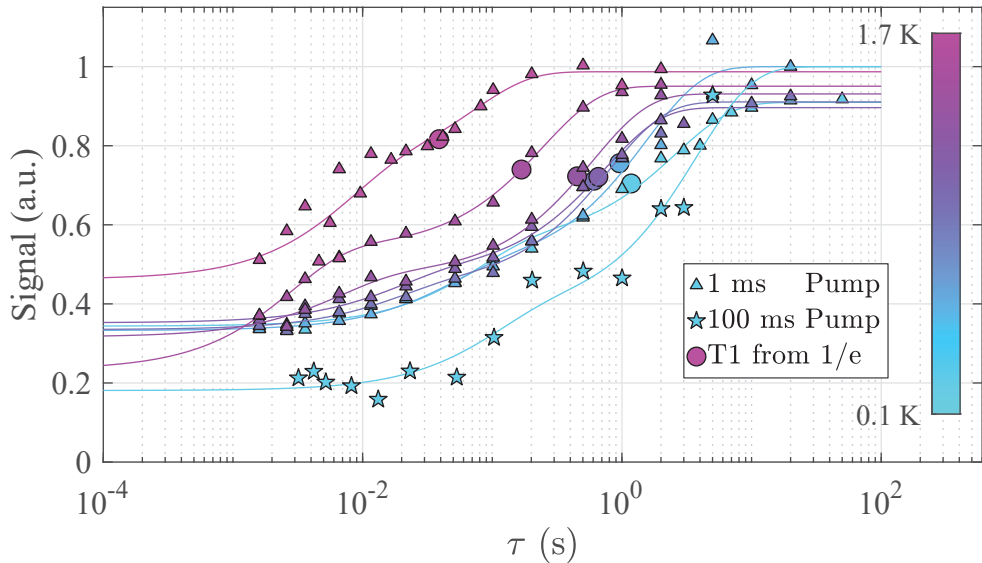

Supplement: Supplementary file 1 [file supplementary_figures.pdf]
